# Supplementary material for: Low Lattice Thermal Conductivity of a Two-Dimensional Phosphorene Oxide
Source: arXiv:1811.04612 source file (2019-03-14)
Supplement: Supplementary file 1 [file SI.pdf]

# **Low Lattice Thermal Conductivity of a Two-Dimensional Phosphorene Oxide**

Seungjun Lee,<sup>1</sup> Seung-Hun Kang,<sup>1,\*</sup> and Young-Kyun Kwon<sup>1,†</sup>

<sup>1</sup>*Department of Physics and Research Institute for Basic Sciences,  
Kyung Hee University, Seoul, 02447, Korea*

(Dated: February 24, 2019)

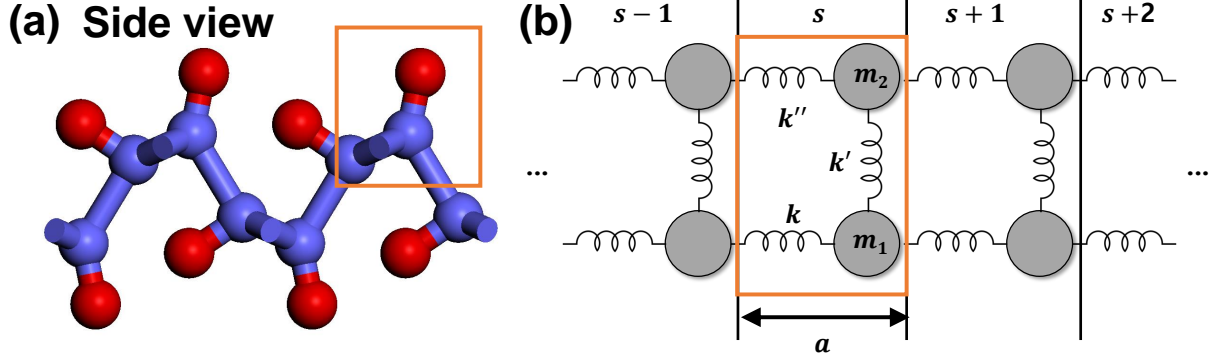

FIG. S1. (a) Side view of phosphorene oxide (PO) and (b) a simple quasi one-dimensional model structure corresponding to PO. Masses  $m_1$  and  $m_2$  represent phosphorous and oxygen atoms, respectively, and the spring constants  $k$ ,  $k'$  and  $k''$  do the P–P, P–O, and O–O bonds, respectively. In the limit of  $k'' \rightarrow 0$ ,  $m_2$  may be mapped into the “flexible” oxygen atom in PO. The box depicts the  $s$ -th unit cell with the lattice constant  $a$  of the mode structure. To simplify the model calculation, we only allowed  $m_1$  and  $m_2$  to move horizontally.

To investigate the role of the “flexible” oxygen atom in PO, we devised the model structure composed of two masses  $m_1$  and  $m_2$  connected with three different types of springs  $k$ ,  $k'$ ,  $k''$  as shown in Fig. S1. With the generalized coordinates  $u_s$  and  $v_s$  assigned to the displacements of the  $s$ -th  $m_1$  and  $m_2$ , the equation of motion is given by

$$m_1 \frac{d^2 u_s}{dt^2} = k(u_{s+1} + u_{s-1} - 2u_s) - k'(u_s - v_s) \quad (\text{S1})$$

$$m_2 \frac{d^2 v_s}{dt^2} = k''(v_{s+1} + v_{s-1} - 2v_s) + k'(u_s - v_s). \quad (\text{S2})$$

We look for a traveling wave solution with different amplitudes  $u$  and  $v$ ,

$$u_s = u e^{i s q a} e^{-i \omega t}, \quad v_s = v e^{i s q a} e^{-i \omega t}.$$

Thus, Eqs. (S1) and (S2) become

$$\begin{aligned} -m_1 \omega^2 u &= k(e^{i q a} + e^{-i q a} - 2)u - k'(u - v) \\ -m_2 \omega^2 v &= k''(e^{i q a} + e^{-i q a} - 2)v + k'(u - v). \end{aligned}$$

These coupled equations can be solved by setting the determinant to be zero, or

$$m_1 m_2 \omega^4 + \omega^2 \left\{ -4(m_2 k + m_1 k'') \sin^2 \left( \frac{qa}{2} \right) - k'(m_1 + m_2) \right\} + 16k k'' \sin^4 \left( \frac{qa}{2} \right) + 4k'(k + k'') \sin^2 \left( \frac{qa}{2} \right) = 0,$$

and thus the two solutions are

$$\begin{aligned} \omega_{\pm}^2 = & 2 \left( \frac{k}{m_1} + \frac{k''}{m_2} \right) \sin^2 \left( \frac{qa}{2} \right) + \frac{k'}{2} \left( \frac{1}{m_1} + \frac{1}{m_2} \right) \\ & \pm \sqrt{4 \left( \frac{k}{m_1} - \frac{k''}{m_2} \right)^2 \sin^4 \left( \frac{qa}{2} \right) + \frac{k'^2}{4} \left( \frac{1}{m_1} + \frac{1}{m_2} \right)^2 + 2k' \sin^2 \left( \frac{qa}{2} \right) \left( \frac{k}{m_1^2} + \frac{k''}{m_2^2} - \frac{k + k''}{m_1 m_2} \right)} \end{aligned} \quad (\text{S3})$$

These solution can be confirmed in a special condition of  $m_1 = m_2 = m$  to be

$$\omega_{\pm}^2 = \frac{1}{m} \left[ 2(k + k'') \sin^2 \left( \frac{qa}{2} \right) + k' \pm \sqrt{4(k - k'')^2 \sin^4 \left( \frac{qa}{2} \right) + k'^2} \right],$$

and further to be, when  $k'' = k$ ,

$$\omega_{\pm}^2 = \frac{1}{m} \left[ 4k \sin^2 \left( \frac{qa}{2} \right) + k' \pm k' \right].$$

The lower solution  $\omega_-$  simply corresponds to the acoustic phonon branch of the monatomic chain system.

To understand role of the flexible oxygen atom corresponding to  $m_2$  and  $k''$ , we plotted the phonon dispersion relations of our model system with various parameters shown in Fig. S2. As clearly seen in the figure, the smaller  $k''$ , the lower the acoustic phonon frequency. Thus, the flexibility of oxygen atoms in PO may lead to the softening of acoustic phonon modes resulting in the reduction in thermal conductivity.

---

\* Current address: Korea Institute for Advanced Study (KIAS), Seoul 02455, Korea

† Corresponding author. E-mail: ykkwon@khu.ac.kr

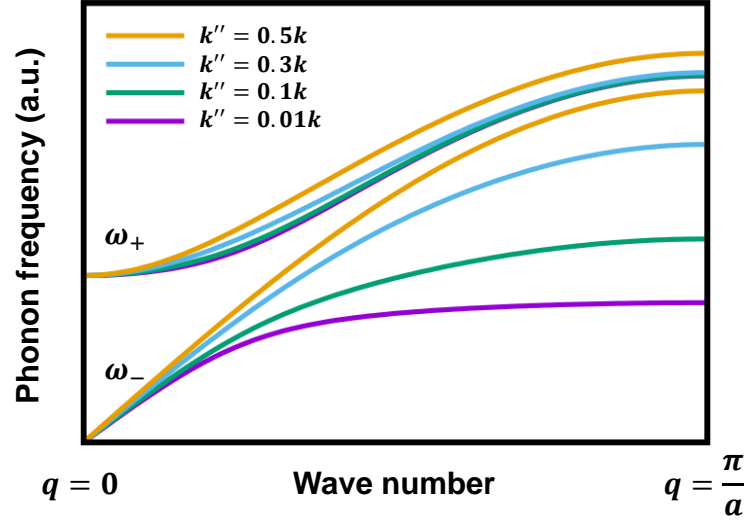

FIG. S2. Calculated phonon dispersion relations of the model system shown in Fig. S1.  $\omega_{\pm}$  given in Eq. S3 represent the optical (+) and acoustic (−) branches, which were plotted with  $m_2 = 0.5m_1$ ,  $k' = 0.3k$ , while changing  $k''$  from  $0.01k$  to  $0.5k$ .
